# Supplementary material for: Optimal exact tests for multiple binary endpoints
Source: arXiv:1612.07561 ancillary file (2016-12-22)
Supplement: Supplementary file 1 [file Supplement_1_Simulation_results_for_two_binary_endpoints.pdf]

# Supplemental material 1

## Simulation results for two binary endpoints

The supplemental tables S1 to S19 show the power for the different closed testing procedures when comparing two treatment groups with respect to two binary endpoints. The tables show the probabilities in percent that the closed testing procedure rejects the global intersection hypothesis  $H_1 \cap H_2$ , at least one elementary null hypothesis ( $H_1$  or  $H_2$ ), both elementary null hypothesis ( $H_1$  and  $H_2$ ), or particularly  $H_1$ , or  $H_2$ .

The unconditional power was calculated numerically for the scenarios with two endpoints. To this end, the rejection region of each test was calculated for all possible row margins  $\tilde{\mathbf{m}}$  (see Section 3 of the manuscript for notation). The corresponding rejection probability under the specified alternative and conditional on  $\tilde{\mathbf{m}}$  was calculated from the conditional joint distribution of the test statistics as given by equation (8) in the manuscript. The unconditional power was then calculated as the weighted sum of the conditional power values, with weights equal to the probability to observe the respective row margins  $\tilde{\mathbf{m}}$ . With two endpoints, the number of possible row margin vectors is  $(2n + 1)^3/6 + (2n + 1)^2/2 + (2n + 1)/3$ . The maximal number of iterations in the branch and bound algorithm was set to 20000. (The algorithm requires approximately 1 second of computation time for 10000 iterations at a 2.4 GHZ CPU.) The optimal solution was found within this number of iterations, except for a few instances in scenarios with  $n = 15$  or  $n = 20$ . For these rare cases the best feasible solution available after the maximal number of iterations was used to define the rejection region.

In the table headings,  $n$  is the sample size per group,  $\alpha$  the nominal familywise significance level,  $p_{i,Trt}$  and  $p_{i,Ctr}$  the success probability in endpoint  $i$  in the treatment and control group, respectively, and  $\rho$  the common product moment correlation between the endpoints.  $p_{i,Trt}$  and  $p_{i,Ctr}$  were chosen such that for efficacious endpoints  $(p_{i,Trt} + p_{i,Ctr})/2 = 0.5$  and the power to reject the hypothesis at an unadjusted level  $\alpha$  using a single Fisher's exact test is approximately 0.6. This way of setting the marginal success rates was chosen in order to obtain scenarios that would be reasonable in a real trial and to allow for comparison of the results across different settings for  $n$  and  $\alpha$ .

The number of instances in which a confirmed optimal solution was found or not found by the branch and bound algorithm, respectively, is given in the two columns labelled C (optimization complete) and NC (not complete). To further quantify the number of required iterations, the median (q50), the 90 % quantile (q90) and the maximum of the number of iterations is shown in the last three columns. A value of 20000 indicates that the respective quantity to achieve an optimal solution would be above 20000, but is here bounded by the maximal number of iterations.

For tests optimizing the power, the assumed alternative is indicated in brackets next

to the test label. There, “all” and “EP 1” refer to an assumed effect identical to the true effect in a scenario with effect in both endpoints or one endpoint, respectively.  $\rho$  there indicates the assumed correlation between the endpoints.

Table S1: Power with two binary endpoints,  $n = 5$ ,  $\alpha = 0.025$ ,  $p_{1,Trt} = 0.865$ ,  $p_{2,Trt} = 0.135$ ,  $p_{1,Ctr} = 0.135$ ,  $p_{2,Ctr} = 0.135$ ,  $\rho = 0$ .

| Test                                         | $H_1 \cap H_2$ | $H_1$ or $H_2$ | $H_1$ and $H_2$ | $H_1$ | $H_2$ | C   | NC | q50 | q90 | Max |
|----------------------------------------------|----------------|----------------|-----------------|-------|-------|-----|----|-----|-----|-----|
| Bonferroni                                   | 23.5           | 23.5           | 0               | 23.5  | 0     |     |    |     |     |     |
| HKT                                          | 58.8           | 58.8           | 0               | 58.8  | 0     |     |    |     |     |     |
| Bonferroni optimal alpha                     | 59.4           | 59.4           | 0               | 59.4  | 0.1   |     |    |     |     |     |
| Bonferroni optimal power (all)               | 59.4           | 59.4           | 0               | 59.4  | 0.1   |     |    |     |     |     |
| Bonferroni optimal power (1)                 | 60.1           | 60.1           | 0               | 60.1  | 0.1   |     |    |     |     |     |
| Bonferroni greedy algorithm                  | 59.3           | 59.3           | 0               | 59.3  | 0.1   |     |    |     |     |     |
| minP                                         | 58.8           | 58.8           | 0               | 58.8  | 0     |     |    |     |     |     |
| Optimal alpha                                | 60.2           | 58.4           | 0               | 58.3  | 0.1   | 286 | 0  | 0   | 3   | 8   |
| Optimal area                                 | 61.8           | 60.1           | 0               | 60.1  | 0.1   | 286 | 0  | 0   | 3   | 8   |
| Optimal power (all, $\rho = 0$ )             | 57             | 55.2           | 0               | 55.1  | 0.1   | 286 | 0  | 0   | 3   | 8   |
| Optimal power (all, $\rho = 0.5$ )           | 57             | 55.2           | 0               | 55.1  | 0.1   | 286 | 0  | 0   | 2   | 4   |
| Optimal power (EP 1, $\rho = 0$ )            | 61.9           | 60.1           | 0               | 60.1  | 0.1   | 286 | 0  | 0   | 3   | 8   |
| Consonant optimal alpha                      | 59.4           | 59.4           | 0               | 59.4  | 0.1   | 286 | 0  | 0   | 3   | 7   |
| Consonnat optimal area                       | 60.1           | 60.1           | 0               | 60.1  | 0.1   | 286 | 0  | 0   | 2   | 7   |
| Consonant optimal power (all, $\rho = 0$ )   | 59.6           | 59.6           | 0               | 59.6  | 0.1   | 286 | 0  | 0   | 2   | 7   |
| Consonant optimal power (all, $\rho = 0.5$ ) | 59.6           | 59.6           | 0               | 59.6  | 0.1   | 286 | 0  | 0   | 2   | 3   |
| Consonant optimal power (EP 1, $\rho = 0$ )  | 60.1           | 60.1           | 0               | 60.1  | 0.1   | 286 | 0  | 0   | 2   | 7   |
| Greedy algorithm                             | 60.9           | 59.2           | 0               | 59.1  | 0.1   |     |    |     |     |     |

Table S2: Power with two binary endpoints,  $n = 5$ ,  $\alpha = 0.025$ ,  $p_{1,Trt} = 0.865$ ,  $p_{2,Trt} = 0.865$ ,  $p_{1,Ctr} = 0.135$ ,  $p_{2,Ctr} = 0.135$ ,  $\rho = 0$ .

| Test                                         | $H_1 \cap H_2$ | $H_1$ or $H_2$ | $H_1$ and $H_2$ | $H_1$ | $H_2$ | C   | NC | q50 | q90 | Max |
|----------------------------------------------|----------------|----------------|-----------------|-------|-------|-----|----|-----|-----|-----|
| Bonferroni                                   | 41.4           | 41.4           | 22.7            | 32    | 32    |     |    |     |     |     |
| HKT                                          | 52.3           | 52.3           | 22.7            | 37.5  | 37.5  |     |    |     |     |     |
| Bonferroni optimal alpha                     | 76.2           | 76.2           | 36.1            | 57.9  | 54.4  |     |    |     |     |     |
| Bonferroni optimal power (all)               | 76.2           | 76.2           | 36.1            | 57.9  | 54.4  |     |    |     |     |     |
| Bonferroni optimal power (1)                 | 72.7           | 72.7           | 36.1            | 60.1  | 48.7  |     |    |     |     |     |
| Bonferroni greedy algorithm                  | 69.1           | 69.1           | 36.1            | 53.4  | 51.7  |     |    |     |     |     |
| minP                                         | 55.7           | 55.7           | 24              | 39.9  | 39.9  |     |    |     |     |     |
| Optimal alpha                                | 81.5           | 75.9           | 36.1            | 57.8  | 54.1  | 286 | 0  | 0   | 3   | 8   |
| Optimal area                                 | 83.3           | 78.2           | 36.1            | 60.1  | 54.2  | 286 | 0  | 0   | 3   | 8   |
| Optimal power (all, $\rho = 0$ )             | 88.3           | 81.2           | 36.1            | 58.9  | 58.3  | 286 | 0  | 0   | 3   | 8   |
| Optimal power (all, $\rho = 0.5$ )           | 88.3           | 81.2           | 36.1            | 58.9  | 58.3  | 286 | 0  | 0   | 2   | 4   |
| Optimal power (EP 1, $\rho = 0$ )            | 83.4           | 78             | 36.1            | 60.1  | 54    | 286 | 0  | 0   | 3   | 8   |
| Consonant optimal alpha                      | 76.2           | 76.2           | 36.1            | 57.9  | 54.4  | 286 | 0  | 0   | 3   | 7   |
| Consonnat optimal area                       | 78.2           | 78.2           | 36.1            | 60.1  | 54.2  | 286 | 0  | 0   | 2   | 7   |
| Consonant optimal power (all, $\rho = 0$ )   | 82.4           | 82.4           | 36.1            | 59.6  | 58.9  | 286 | 0  | 0   | 2   | 7   |
| Consonant optimal power (all, $\rho = 0.5$ ) | 82.4           | 82.4           | 36.1            | 59.6  | 58.9  | 286 | 0  | 0   | 2   | 3   |
| Consonant optimal power (EP 1, $\rho = 0$ )  | 78.2           | 78.2           | 36.1            | 60.1  | 54.2  | 286 | 0  | 0   | 2   | 7   |
| Greedy algorithm                             | 86.3           | 81.1           | 36.1            | 59.8  | 57.4  |     |    |     |     |     |

Table S3: Power with two binary endpoints,  $n = 5$ ,  $\alpha = 0.025$ ,  $p_{1,Trt} = 0.865$ ,  $p_{2,Trt} = 0.865$ ,  $p_{1,Ctr} = 0.135$ ,  $p_{2,Ctr} = 0.135$ ,  $\rho = 0.5$ .

| Test                                         | $H_1 \cap H_2$ | $H_1$ or $H_2$ | $H_1$ and $H_2$ | $H_1$ | $H_2$ | C   | NC | q50 | q90 | Max |
|----------------------------------------------|----------------|----------------|-----------------|-------|-------|-----|----|-----|-----|-----|
| Bonferroni                                   | 35.2           | 35.2           | 28.5            | 31.9  | 31.9  |     |    |     |     |     |
| HKT                                          | 44.3           | 44.3           | 28.5            | 36.4  | 36.4  |     |    |     |     |     |
| Bonferroni optimal alpha                     | 72.1           | 72.1           | 45.1            | 59.6  | 57.6  |     |    |     |     |     |
| Bonferroni optimal power (all)               | 72.1           | 72.1           | 45.1            | 59.6  | 57.6  |     |    |     |     |     |
| Bonferroni optimal power (1)                 | 67.5           | 67.5           | 45.1            | 60.1  | 52.5  |     |    |     |     |     |
| Bonferroni greedy algorithm                  | 62.8           | 62.8           | 45.1            | 54.6  | 53.3  |     |    |     |     |     |
| minP                                         | 63.4           | 63.4           | 39.6            | 51.5  | 51.5  |     |    |     |     |     |
| Optimal alpha                                | 73.3           | 72.1           | 45.1            | 59.6  | 57.6  | 286 | 0  | 0   | 3   | 8   |
| Optimal area                                 | 73.6           | 72.4           | 45.1            | 60.1  | 57.4  | 286 | 0  | 0   | 3   | 8   |
| Optimal power (all, $\rho = 0$ )             | 74.1           | 72.8           | 45.1            | 59.5  | 58.4  | 286 | 0  | 0   | 3   | 8   |
| Optimal power (all, $\rho = 0.5$ )           | 74.1           | 72.8           | 45.1            | 59.5  | 58.4  | 286 | 0  | 0   | 2   | 4   |
| Optimal power (EP 1, $\rho = 0$ )            | 73.6           | 72.4           | 45.1            | 60.1  | 57.4  | 286 | 0  | 0   | 3   | 8   |
| Consonant optimal alpha                      | 72.1           | 72.1           | 45.1            | 59.6  | 57.6  | 286 | 0  | 0   | 3   | 7   |
| Consonnat optimal area                       | 72.4           | 72.4           | 45.1            | 60.1  | 57.4  | 286 | 0  | 0   | 2   | 7   |
| Consonant optimal power (all, $\rho = 0$ )   | 72.9           | 72.9           | 45.1            | 59.6  | 58.4  | 286 | 0  | 0   | 2   | 7   |
| Consonant optimal power (all, $\rho = 0.5$ ) | 72.9           | 72.9           | 45.1            | 59.6  | 58.4  | 286 | 0  | 0   | 2   | 3   |
| Consonant optimal power (EP 1, $\rho = 0$ )  | 72.4           | 72.4           | 45.1            | 60.1  | 57.4  | 286 | 0  | 0   | 2   | 7   |
| Greedy algorithm                             | 74             | 72.7           | 45.1            | 59.9  | 58    |     |    |     |     |     |

Table S4: Power with two binary endpoints,  $n = 10$ ,  $\alpha = 0.025$ ,  $p_{1,Trt} = 0.792$ ,  $p_{2,Trt} = 0.208$ ,  $p_{1,Ctr} = 0.208$ ,  $p_{2,Ctr} = 0.208$ ,  $\rho = 0$ .

| Test                                         | $H_1 \cap H_2$ | $H_1$ or $H_2$ | $H_1$ and $H_2$ | $H_1$ | $H_2$ | C    | NC | q50 | q90 | Max |
|----------------------------------------------|----------------|----------------|-----------------|-------|-------|------|----|-----|-----|-----|
| Bonferroni                                   | 59.5           | 59.5           | 0.2             | 59.5  | 0.3   |      |    |     |     |     |
| HKT                                          | 59.9           | 59.9           | 0.2             | 59.8  | 0.3   |      |    |     |     |     |
| Bonferroni optimal alpha                     | 56.6           | 56.6           | 0.2             | 56.5  | 0.4   |      |    |     |     |     |
| Bonferroni optimal power (all)               | 56.6           | 56.6           | 0.2             | 56.5  | 0.4   |      |    |     |     |     |
| Bonferroni optimal power (1)                 | 60.2           | 60.2           | 0.2             | 60.1  | 0.4   |      |    |     |     |     |
| Bonferroni greedy algorithm                  | 60.2           | 60.2           | 0.2             | 60    | 0.4   |      |    |     |     |     |
| minP                                         | 60.1           | 60.1           | 0.2             | 59.9  | 0.4   |      |    |     |     |     |
| Optimal alpha                                | 56.9           | 49.4           | 0.2             | 49.3  | 0.4   | 1771 | 0  | 4   | 25  | 81  |
| Optimal area                                 | 67.1           | 60             | 0.2             | 59.8  | 0.4   | 1771 | 0  | 4   | 24  | 78  |
| Optimal power (all, $\rho = 0$ )             | 57.7           | 50.7           | 0.2             | 50.5  | 0.4   | 1771 | 0  | 3   | 42  | 186 |
| Optimal power (all, $\rho = 0.5$ )           | 57.6           | 50.5           | 0.2             | 50.4  | 0.4   | 1771 | 0  | 2   | 8   | 22  |
| Optimal power (EP 1, $\rho = 0$ )            | 70             | 60.2           | 0.2             | 60    | 0.4   | 1771 | 0  | 3   | 58  | 275 |
| Consonant optimal alpha                      | 60             | 60             | 0.2             | 59.8  | 0.4   | 1771 | 0  | 0   | 0   | 18  |
| Consonnat optimal area                       | 60             | 60             | 0.2             | 59.8  | 0.4   | 1771 | 0  | 0   | 0   | 18  |
| Consonant optimal power (all, $\rho = 0$ )   | 60             | 60             | 0.2             | 59.9  | 0.4   | 1771 | 0  | 0   | 0   | 21  |
| Consonant optimal power (all, $\rho = 0.5$ ) | 60             | 60             | 0.2             | 59.9  | 0.4   | 1771 | 0  | 0   | 0   | 10  |
| Consonant optimal power (EP 1, $\rho = 0$ )  | 60.2           | 60.2           | 0.2             | 60.1  | 0.4   | 1771 | 0  | 0   | 0   | 21  |
| Greedy algorithm                             | 65.7           | 60.2           | 0.2             | 60    | 0.4   |      |    |     |     |     |

Table S5: Power with two binary endpoints,  $n = 10$ ,  $\alpha = 0.025$ ,  $p_{1,Trt} = 0.792$ ,  $p_{2,Trt} = 0.792$ ,  $p_{1,Ctr} = 0.208$ ,  $p_{2,Ctr} = 0.208$ ,  $\rho = 0$ .

| Test                                         | $H_1 \cap H_2$ | $H_1$ or $H_2$ | $H_1$ and $H_2$ | $H_1$ | $H_2$ | C    | NC | q50 | q90 | Max |
|----------------------------------------------|----------------|----------------|-----------------|-------|-------|------|----|-----|-----|-----|
| Bonferroni                                   | 83.6           | 83.6           | 36.1            | 59.8  | 59.8  |      |    |     |     |     |
| HKT                                          | 83.6           | 83.6           | 36.1            | 59.8  | 59.8  |      |    |     |     |     |
| Bonferroni optimal alpha                     | 83.9           | 83.9           | 36.1            | 60    | 60    |      |    |     |     |     |
| Bonferroni optimal power (all)               | 83.9           | 83.9           | 36.1            | 60    | 60    |      |    |     |     |     |
| Bonferroni optimal power (1)                 | 83.9           | 83.9           | 36.1            | 60.1  | 59.9  |      |    |     |     |     |
| Bonferroni greedy algorithm                  | 83.9           | 83.9           | 36.1            | 60    | 60    |      |    |     |     |     |
| minP                                         | 83.9           | 83.9           | 36.1            | 60    | 60    |      |    |     |     |     |
| Optimal alpha                                | 94.3           | 82.6           | 36.1            | 59.5  | 59.2  | 1771 | 0  | 4   | 25  | 81  |
| Optimal area                                 | 94.3           | 84             | 36.1            | 60.1  | 60    | 1771 | 0  | 4   | 24  | 78  |
| Optimal power (all, $\rho = 0$ )             | 96.2           | 83.7           | 36.1            | 59.9  | 59.9  | 1771 | 0  | 3   | 42  | 186 |
| Optimal power (all, $\rho = 0.5$ )           | 96.2           | 83.7           | 36.1            | 59.9  | 59.9  | 1771 | 0  | 2   | 8   | 22  |
| Optimal power (EP 1, $\rho = 0$ )            | 94.2           | 83             | 36.1            | 60.1  | 59    | 1771 | 0  | 3   | 58  | 275 |
| Consonant optimal alpha                      | 84             | 84             | 36.1            | 60.1  | 60.1  | 1771 | 0  | 0   | 0   | 18  |
| Consonnat optimal area                       | 84             | 84             | 36.1            | 60.1  | 60.1  | 1771 | 0  | 0   | 0   | 18  |
| Consonant optimal power (all, $\rho = 0$ )   | 84             | 84             | 36.1            | 60.1  | 60.1  | 1771 | 0  | 0   | 0   | 21  |
| Consonant optimal power (all, $\rho = 0.5$ ) | 84             | 84             | 36.1            | 60.1  | 60.1  | 1771 | 0  | 0   | 0   | 10  |
| Consonant optimal power (EP 1, $\rho = 0$ )  | 84             | 84             | 36.1            | 60.1  | 60.1  | 1771 | 0  | 0   | 0   | 21  |
| Greedy algorithm                             | 94.4           | 84             | 36.1            | 60.1  | 60.1  |      |    |     |     |     |

Table S6: Power with two binary endpoints,  $n = 10$ ,  $\alpha = 0.025$ ,  $p_{1,Trt} = 0.792$ ,  $p_{2,Trt} = 0.792$ ,  $p_{1,Ctr} = 0.208$ ,  $p_{2,Ctr} = 0.208$ ,  $\rho = 0.5$ .

| Test                                         | $H_1 \cap H_2$ | $H_1$ or $H_2$ | $H_1$ and $H_2$ | $H_1$ | $H_2$ | C    | NC | q50 | q90 | Max |
|----------------------------------------------|----------------|----------------|-----------------|-------|-------|------|----|-----|-----|-----|
| Bonferroni                                   | 75.2           | 75.2           | 44.3            | 59.8  | 59.8  |      |    |     |     |     |
| HKT                                          | 75.2           | 75.2           | 44.3            | 59.8  | 59.8  |      |    |     |     |     |
| Bonferroni optimal alpha                     | 75.7           | 75.7           | 44.3            | 60    | 60    |      |    |     |     |     |
| Bonferroni optimal power (all)               | 75.7           | 75.7           | 44.3            | 60    | 60    |      |    |     |     |     |
| Bonferroni optimal power (1)                 | 75.7           | 75.7           | 44.3            | 60.1  | 59.9  |      |    |     |     |     |
| Bonferroni greedy algorithm                  | 75.7           | 75.7           | 44.3            | 60    | 60    |      |    |     |     |     |
| minP                                         | 75.7           | 75.7           | 44.3            | 60    | 60    |      |    |     |     |     |
| Optimal alpha                                | 84.4           | 74.5           | 44.3            | 59.4  | 59.4  | 1771 | 0  | 4   | 25  | 81  |
| Optimal area                                 | 83.7           | 75.4           | 44.3            | 60.1  | 59.7  | 1771 | 0  | 4   | 24  | 78  |
| Optimal power (all, $\rho = 0$ )             | 84.6           | 74.9           | 44.3            | 59.6  | 59.6  | 1771 | 0  | 3   | 42  | 186 |
| Optimal power (all, $\rho = 0.5$ )           | 84.6           | 74.9           | 44.3            | 59.6  | 59.6  | 1771 | 0  | 2   | 8   | 22  |
| Optimal power (EP 1, $\rho = 0$ )            | 83.6           | 75.2           | 44.3            | 60.1  | 59.5  | 1771 | 0  | 3   | 58  | 275 |
| Consonant optimal alpha                      | 75.8           | 75.8           | 44.3            | 60.1  | 60    | 1771 | 0  | 0   | 0   | 18  |
| Consonnat optimal area                       | 75.8           | 75.8           | 44.3            | 60.1  | 60    | 1771 | 0  | 0   | 0   | 18  |
| Consonant optimal power (all, $\rho = 0$ )   | 75.8           | 75.8           | 44.3            | 60.1  | 60    | 1771 | 0  | 0   | 0   | 21  |
| Consonant optimal power (all, $\rho = 0.5$ ) | 75.8           | 75.8           | 44.3            | 60.1  | 60    | 1771 | 0  | 0   | 0   | 10  |
| Consonant optimal power (EP 1, $\rho = 0$ )  | 75.8           | 75.8           | 44.3            | 60.1  | 60    | 1771 | 0  | 0   | 0   | 21  |
| Greedy algorithm                             | 83             | 75.8           | 44.3            | 60.1  | 60    |      |    |     |     |     |



Table S7: Power with two binary endpoints,  $n = 15$ ,  $\alpha = 0.025$ ,  $p_{1,Trt} = 0.265$ ,  $p_{2,Trt} = 0.265$ ,  $p_{1,Ctr} = 0.265$ ,  $p_{2,Ctr} = 0.265$ ,  $\rho = 0$ .

| Test                                         | $H_1 \cap H_2$ | $H_1$ or $H_2$ | $H_1$ and $H_2$ | $H_1$ | $H_2$ | C    | NC | q50 | q90  | Max   |
|----------------------------------------------|----------------|----------------|-----------------|-------|-------|------|----|-----|------|-------|
| Bonferroni                                   | 0.8            | 0.8            | 0.01            | 0.4   | 0.4   |      |    |     |      |       |
| HKT                                          | 0.92           | 0.92           | 0.01            | 0.46  | 0.46  |      |    |     |      |       |
| Bonferroni optimal alpha                     | 1.53           | 1.53           | 0.01            | 0.8   | 0.74  |      |    |     |      |       |
| Bonferroni optimal power (all)               | 1.53           | 1.53           | 0.01            | 0.75  | 0.78  |      |    |     |      |       |
| Bonferroni optimal power (1)                 | 1.45           | 1.45           | 0.01            | 0.88  | 0.58  |      |    |     |      |       |
| Bonferroni greedy algorithm                  | 1.38           | 1.38           | 0.01            | 0.72  | 0.66  |      |    |     |      |       |
| minP                                         | 1.32           | 1.32           | 0.01            | 0.66  | 0.66  |      |    |     |      |       |
| Optimal alpha                                | 2.44           | 1.03           | 0.01            | 0.54  | 0.49  | 5456 | 0  | 17  | 137  | 889   |
| Optimal area                                 | 2.21           | 1.55           | 0.01            | 0.86  | 0.71  | 5456 | 0  | 17  | 136  | 874   |
| Optimal power (all, $\rho = 0$ )             | 2.36           | 0.88           | 0.01            | 0.45  | 0.43  | 5456 | 0  | 37  | 649  | 4438  |
| Optimal power (all, $\rho = 0.5$ )           | 2.37           | 0.86           | 0.01            | 0.45  | 0.42  | 5456 | 0  | 8   | 43   | 143   |
| Optimal power (EP 1, $\rho = 0$ )            | 2.33           | 1.18           | 0.01            | 0.87  | 0.32  | 5456 | 0  | 43  | 1765 | 14350 |
| Consonant optimal alpha                      | 1.61           | 1.61           | 0.01            | 0.82  | 0.8   | 5456 | 0  | 0   | 7    | 68    |
| Consonnat optimal area                       | 1.59           | 1.59           | 0.01            | 0.86  | 0.73  | 5456 | 0  | 0   | 7    | 68    |
| Consonant optimal power (all, $\rho = 0$ )   | 1.6            | 1.6            | 0.01            | 0.81  | 0.8   | 5456 | 0  | 0   | 7    | 226   |
| Consonant optimal power (all, $\rho = 0.5$ ) | 1.6            | 1.6            | 0.01            | 0.81  | 0.8   | 5456 | 0  | 0   | 3    | 45    |
| Consonant optimal power (EP 1, $\rho = 0$ )  | 1.59           | 1.59           | 0.01            | 0.88  | 0.72  | 5456 | 0  | 0   | 7    | 242   |
| Greedy algorithm                             | 2.12           | 1.47           | 0.01            | 0.76  | 0.72  |      |    |     |      |       |

Table S8: Power with two binary endpoints,  $n = 15$ ,  $\alpha = 0.025$ ,  $p_{1,Trt} = 0.265$ ,  $p_{2,Trt} = 0.265$ ,  $p_{1,Ctr} = 0.265$ ,  $p_{2,Ctr} = 0.265$ ,  $\rho = 0.5$ .

| Test                                         | $H_1 \cap H_2$ | $H_1$ or $H_2$ | $H_1$ and $H_2$ | $H_1$ | $H_2$ | C    | NC | q50 | q90  | Max   |
|----------------------------------------------|----------------|----------------|-----------------|-------|-------|------|----|-----|------|-------|
| Bonferroni                                   | 0.77           | 0.77           | 0.08            | 0.43  | 0.43  |      |    |     |      |       |
| HKT                                          | 0.89           | 0.89           | 0.09            | 0.49  | 0.49  |      |    |     |      |       |
| Bonferroni optimal alpha                     | 1.47           | 1.47           | 0.1             | 0.82  | 0.75  |      |    |     |      |       |
| Bonferroni optimal power (all)               | 1.47           | 1.47           | 0.1             | 0.78  | 0.79  |      |    |     |      |       |
| Bonferroni optimal power (1)                 | 1.41           | 1.41           | 0.1             | 0.88  | 0.63  |      |    |     |      |       |
| Bonferroni greedy algorithm                  | 1.34           | 1.34           | 0.1             | 0.76  | 0.69  |      |    |     |      |       |
| minP                                         | 1.33           | 1.33           | 0.09            | 0.71  | 0.71  |      |    |     |      |       |
| Optimal alpha                                | 2.21           | 1.29           | 0.1             | 0.72  | 0.68  | 5456 | 0  | 17  | 137  | 889   |
| Optimal area                                 | 2.04           | 1.52           | 0.1             | 0.86  | 0.76  | 5456 | 0  | 17  | 136  | 874   |
| Optimal power (all, $\rho = 0$ )             | 2.14           | 1.23           | 0.1             | 0.68  | 0.65  | 5456 | 0  | 37  | 649  | 4438  |
| Optimal power (all, $\rho = 0.5$ )           | 2.15           | 1.24           | 0.1             | 0.69  | 0.66  | 5456 | 0  | 8   | 43   | 143   |
| Optimal power (EP 1, $\rho = 0$ )            | 2.1            | 1.33           | 0.1             | 0.88  | 0.56  | 5456 | 0  | 43  | 1765 | 14350 |
| Consonant optimal alpha                      | 1.54           | 1.54           | 0.1             | 0.83  | 0.81  | 5456 | 0  | 0   | 7    | 68    |
| Consonnat optimal area                       | 1.53           | 1.53           | 0.1             | 0.86  | 0.77  | 5456 | 0  | 0   | 7    | 68    |
| Consonant optimal power (all, $\rho = 0$ )   | 1.53           | 1.53           | 0.1             | 0.83  | 0.81  | 5456 | 0  | 0   | 7    | 226   |
| Consonant optimal power (all, $\rho = 0.5$ ) | 1.53           | 1.53           | 0.1             | 0.83  | 0.81  | 5456 | 0  | 0   | 3    | 45    |
| Consonant optimal power (EP 1, $\rho = 0$ )  | 1.52           | 1.52           | 0.1             | 0.88  | 0.75  | 5456 | 0  | 0   | 7    | 242   |
| Greedy algorithm                             | 1.96           | 1.51           | 0.1             | 0.83  | 0.78  |      |    |     |      |       |

Table S9: Power with two binary endpoints,  $n = 15$ ,  $\alpha = 0.025$ ,  $p_{1,Trt} = 0.735$ ,  $p_{2,Trt} = 0.265$ ,  $p_{1,Ctr} = 0.265$ ,  $p_{2,Ctr} = 0.265$ ,  $\rho = 0$ .

| Test                                         | $H_1 \cap H_2$ | $H_1$ or $H_2$ | $H_1$ and $H_2$ | $H_1$ | $H_2$ | C    | NC | q50 | q90  | Max   |
|----------------------------------------------|----------------|----------------|-----------------|-------|-------|------|----|-----|------|-------|
| Bonferroni                                   | 47.6           | 47.6           | 0.5             | 47.5  | 0.6   |      |    |     |      |       |
| HKT                                          | 49.6           | 49.6           | 0.5             | 49.5  | 0.7   |      |    |     |      |       |
| Bonferroni optimal alpha                     | 56             | 56             | 0.5             | 55.7  | 0.9   |      |    |     |      |       |
| Bonferroni optimal power (all)               | 55.9           | 55.9           | 0.5             | 55.6  | 0.9   |      |    |     |      |       |
| Bonferroni optimal power (1)                 | 60.6           | 60.6           | 0.5             | 60.4  | 0.8   |      |    |     |      |       |
| Bonferroni greedy algorithm                  | 60.5           | 60.5           | 0.5             | 60.2  | 0.8   |      |    |     |      |       |
| minP                                         | 60.3           | 60.3           | 0.5             | 60.1  | 0.8   |      |    |     |      |       |
| Optimal alpha                                | 47             | 40.6           | 0.5             | 40.3  | 0.9   | 5456 | 0  | 17  | 137  | 889   |
| Optimal area                                 | 63.8           | 58.9           | 0.5             | 58.6  | 0.9   | 5456 | 0  | 17  | 136  | 874   |
| Optimal power (all, $\rho = 0$ )             | 53.6           | 46.9           | 0.5             | 46.6  | 0.9   | 5456 | 0  | 37  | 649  | 4438  |
| Optimal power (all, $\rho = 0.5$ )           | 52.8           | 46             | 0.5             | 45.7  | 0.9   | 5456 | 0  | 8   | 43   | 143   |
| Optimal power (EP 1, $\rho = 0$ )            | 70.9           | 60.4           | 0.5             | 60.1  | 0.8   | 5456 | 0  | 43  | 1765 | 14350 |
| Consonant optimal alpha                      | 58.9           | 58.9           | 0.5             | 58.5  | 0.9   | 5456 | 0  | 0   | 7    | 68    |
| Consonnat optimal area                       | 58.8           | 58.8           | 0.5             | 58.4  | 0.9   | 5456 | 0  | 0   | 7    | 68    |
| Consonant optimal power (all, $\rho = 0$ )   | 60.2           | 60.2           | 0.5             | 59.9  | 0.9   | 5456 | 0  | 0   | 7    | 226   |
| Consonant optimal power (all, $\rho = 0.5$ ) | 60.2           | 60.2           | 0.5             | 59.9  | 0.9   | 5456 | 0  | 0   | 3    | 45    |
| Consonant optimal power (EP 1, $\rho = 0$ )  | 60.7           | 60.7           | 0.5             | 60.4  | 0.9   | 5456 | 0  | 0   | 7    | 242   |
| Greedy algorithm                             | 64.2           | 60.4           | 0.5             | 60    | 0.9   |      |    |     |      |       |

Table S10: Power with two binary endpoints,  $n = 15$ ,  $\alpha = 0.025$ ,  $p_{1,Trt} = 0.735$ ,  $p_{2,Trt} = 0.735$ ,  $p_{1,Ctr} = 0.265$ ,  $p_{2,Ctr} = 0.265$ ,  $\rho = 0$ .

| Test                                         | $H_1 \cap H_2$ | $H_1$ or $H_2$ | $H_1$ and $H_2$ | $H_1$ | $H_2$ | C    | NC | q50 | q90  | Max   |
|----------------------------------------------|----------------|----------------|-----------------|-------|-------|------|----|-----|------|-------|
| Bonferroni                                   | 72.3           | 72.3           | 34.8            | 53.6  | 53.6  |      |    |     |      |       |
| HKT                                          | 72.3           | 72.3           | 34.8            | 53.6  | 53.6  |      |    |     |      |       |
| Bonferroni optimal alpha                     | 82.7           | 82.7           | 36.5            | 60    | 59.2  |      |    |     |      |       |
| Bonferroni optimal power (all)               | 82.7           | 82.7           | 36.5            | 60    | 59.2  |      |    |     |      |       |
| Bonferroni optimal power (1)                 | 82.7           | 82.7           | 36.5            | 60.4  | 58.8  |      |    |     |      |       |
| Bonferroni greedy algorithm                  | 82.7           | 82.7           | 36.5            | 59.8  | 59.3  |      |    |     |      |       |
| minP                                         | 81.5           | 81.5           | 35.9            | 58.8  | 58.6  |      |    |     |      |       |
| Optimal alpha                                | 92.6           | 82.3           | 36.5            | 59.5  | 59.3  | 5456 | 0  | 17  | 137  | 889   |
| Optimal area                                 | 93             | 84.3           | 36.5            | 60.4  | 60.4  | 5456 | 0  | 17  | 136  | 874   |
| Optimal power (all, $\rho = 0$ )             | 95.7           | 83.9           | 36.5            | 60.2  | 60.1  | 5456 | 0  | 37  | 649  | 4438  |
| Optimal power (all, $\rho = 0.5$ )           | 95.7           | 83.8           | 36.5            | 60.2  | 60.1  | 5456 | 0  | 8   | 43   | 143   |
| Optimal power (EP 1, $\rho = 0$ )            | 92.2           | 82.4           | 36.5            | 60.4  | 58.5  | 5456 | 0  | 43  | 1765 | 14350 |
| Consonant optimal alpha                      | 84.3           | 84.3           | 36.5            | 60.4  | 60.4  | 5456 | 0  | 0   | 7    | 68    |
| Consonnat optimal area                       | 84.3           | 84.3           | 36.5            | 60.4  | 60.4  | 5456 | 0  | 0   | 7    | 68    |
| Consonant optimal power (all, $\rho = 0$ )   | 84.3           | 84.3           | 36.5            | 60.4  | 60.4  | 5456 | 0  | 0   | 7    | 226   |
| Consonant optimal power (all, $\rho = 0.5$ ) | 84.3           | 84.3           | 36.5            | 60.4  | 60.4  | 5456 | 0  | 0   | 3    | 45    |
| Consonant optimal power (EP 1, $\rho = 0$ )  | 84.3           | 84.3           | 36.5            | 60.4  | 60.4  | 5456 | 0  | 0   | 7    | 242   |
| Greedy algorithm                             | 93.2           | 84.3           | 36.5            | 60.4  | 60.4  |      |    |     |      |       |

Table S11: Power with two binary endpoints,  $n = 15$ ,  $\alpha = 0.025$ ,  $p_{1,T\gamma t} = 0.735$ ,  $p_{2,T\gamma t} = 0.735$ ,  $p_{1,Ctr} = 0.265$ ,  $p_{2,Ctr} = 0.265$ ,  $\rho = 0.5$ .

| Test                                         | $H_1 \cap H_2$ | $H_1$ or $H_2$ | $H_1$ and $H_2$ | $H_1$ | $H_2$ | C    | NC | q50 | q90  | Max   |
|----------------------------------------------|----------------|----------------|-----------------|-------|-------|------|----|-----|------|-------|
| Bonferroni                                   | 64             | 64             | 42.5            | 53.3  | 53.3  |      |    |     |      |       |
| HKT                                          | 64             | 64             | 42.5            | 53.3  | 53.3  |      |    |     |      |       |
| Bonferroni optimal alpha                     | 74.7           | 74.7           | 44.6            | 60    | 59.2  |      |    |     |      |       |
| Bonferroni optimal power (all)               | 74.6           | 74.6           | 44.6            | 60    | 59.2  |      |    |     |      |       |
| Bonferroni optimal power (1)                 | 74.6           | 74.6           | 44.6            | 60.4  | 58.8  |      |    |     |      |       |
| Bonferroni greedy algorithm                  | 74.6           | 74.6           | 44.6            | 59.9  | 59.3  |      |    |     |      |       |
| minP                                         | 75.7           | 75.7           | 44.5            | 60.1  | 60    |      |    |     |      |       |
| Optimal alpha                                | 83.6           | 74.3           | 44.6            | 59.5  | 59.4  | 5456 | 0  | 17  | 137  | 889   |
| Optimal area                                 | 83.4           | 76.1           | 44.6            | 60.4  | 60.2  | 5456 | 0  | 17  | 136  | 874   |
| Optimal power (all, $\rho = 0$ )             | 84.6           | 75.4           | 44.6            | 60    | 59.9  | 5456 | 0  | 37  | 649  | 4438  |
| Optimal power (all, $\rho = 0.5$ )           | 84.6           | 75.4           | 44.6            | 60    | 59.9  | 5456 | 0  | 8   | 43   | 143   |
| Optimal power (EP 1, $\rho = 0$ )            | 83.2           | 75             | 44.6            | 60.4  | 59.2  | 5456 | 0  | 43  | 1765 | 14350 |
| Consonant optimal alpha                      | 76.2           | 76.2           | 44.6            | 60.4  | 60.4  | 5456 | 0  | 0   | 7    | 68    |
| Consonnat optimal area                       | 76.2           | 76.2           | 44.6            | 60.4  | 60.4  | 5456 | 0  | 0   | 7    | 68    |
| Consonant optimal power (all, $\rho = 0$ )   | 76.2           | 76.2           | 44.6            | 60.4  | 60.4  | 5456 | 0  | 0   | 7    | 226   |
| Consonant optimal power (all, $\rho = 0.5$ ) | 76.2           | 76.2           | 44.6            | 60.4  | 60.4  | 5456 | 0  | 0   | 3    | 45    |
| Consonant optimal power (EP 1, $\rho = 0$ )  | 76.2           | 76.2           | 44.6            | 60.4  | 60.4  | 5456 | 0  | 0   | 7    | 242   |
| Greedy algorithm                             | 82.9           | 76.2           | 44.6            | 60.4  | 60.4  |      |    |     |      |       |

Table S12: Power with two binary endpoints,  $n = 15$ ,  $\alpha = 0.05$ ,  $p_{1,Trt} = 0.297$ ,  $p_{2,Trt} = 0.297$ ,  $p_{1,Ctr} = 0.297$ ,  $p_{2,Ctr} = 0.297$ ,  $\rho = 0$ .

| Test                                         | $H_1 \cap H_2$ | $H_1$ or $H_2$ | $H_1$ and $H_2$ | $H_1$ | $H_2$ | C    | NC | q50 | q90   | Max   |
|----------------------------------------------|----------------|----------------|-----------------|-------|-------|------|----|-----|-------|-------|
| Bonferroni                                   | 1.7            | 1.7            | 0.03            | 0.86  | 0.86  |      |    |     |       |       |
| HKT                                          | 1.77           | 1.77           | 0.03            | 0.9   | 0.9   |      |    |     |       |       |
| Bonferroni optimal alpha                     | 3.4            | 3.4            | 0.04            | 1.78  | 1.66  |      |    |     |       |       |
| Bonferroni optimal power (all)               | 3.31           | 3.31           | 0.04            | 1.68  | 1.67  |      |    |     |       |       |
| Bonferroni optimal power (1)                 | 3.18           | 3.18           | 0.04            | 2     | 1.22  |      |    |     |       |       |
| Bonferroni greedy algorithm                  | 2.96           | 2.96           | 0.04            | 1.56  | 1.44  |      |    |     |       |       |
| minP                                         | 2.94           | 2.94           | 0.04            | 1.49  | 1.49  |      |    |     |       |       |
| Optimal alpha                                | 4.96           | 2.39           | 0.04            | 1.25  | 1.18  | 5456 | 0  | 22  | 160.5 | 1002  |
| Optimal area                                 | 4.53           | 3.5            | 0.04            | 1.9   | 1.64  | 5456 | 0  | 22  | 156.5 | 998   |
| Optimal power (all, $\rho = 0$ )             | 4.85           | 2.15           | 0.04            | 1.11  | 1.08  | 5456 | 0  | 55  | 927   | 8955  |
| Optimal power (all, $\rho = 0.5$ )           | 4.86           | 2.17           | 0.04            | 1.12  | 1.09  | 5456 | 0  | 13  | 66    | 241   |
| Optimal power (EP 1, $\rho = 0$ )            | 4.78           | 2.68           | 0.04            | 1.99  | 0.73  | 5454 | 2  | 61  | 2446  | 20000 |
| Consonant optimal alpha                      | 3.65           | 3.65           | 0.04            | 1.87  | 1.83  | 5456 | 0  | 0   | 33    | 206   |
| Consonnat optimal area                       | 3.57           | 3.57           | 0.04            | 1.91  | 1.7   | 5456 | 0  | 0   | 33    | 206   |
| Consonant optimal power (all, $\rho = 0$ )   | 3.61           | 3.61           | 0.04            | 1.83  | 1.82  | 5456 | 0  | 0   | 45    | 1008  |
| Consonant optimal power (all, $\rho = 0.5$ ) | 3.61           | 3.61           | 0.04            | 1.83  | 1.82  | 5456 | 0  | 0   | 8     | 71    |
| Consonant optimal power (EP 1, $\rho = 0$ )  | 3.59           | 3.59           | 0.04            | 2     | 1.63  | 5456 | 0  | 0   | 52.5  | 1122  |
| Greedy algorithm                             | 4.36           | 3.37           | 0.04            | 1.73  | 1.68  |      |    |     |       |       |

Table S13: Power with two binary endpoints,  $n = 15$ ,  $\alpha = 0.05$ ,  $p_{1,Trt} = 0.297$ ,  $p_{2,Trt} = 0.297$ ,  $p_{1,Ctr} = 0.297$ ,  $p_{2,Ctr} = 0.297$ ,  $\rho = 0.5$ .

| Test                                         | $H_1 \cap H_2$ | $H_1$ or $H_2$ | $H_1$ and $H_2$ | $H_1$ | $H_2$ | C    | NC | q50 | q90   | Max   |
|----------------------------------------------|----------------|----------------|-----------------|-------|-------|------|----|-----|-------|-------|
| Bonferroni                                   | 1.6            | 1.6            | 0.25            | 0.93  | 0.93  |      |    |     |       |       |
| HKT                                          | 1.67           | 1.67           | 0.26            | 0.96  | 0.96  |      |    |     |       |       |
| Bonferroni optimal alpha                     | 3.23           | 3.23           | 0.33            | 1.85  | 1.71  |      |    |     |       |       |
| Bonferroni optimal power (all)               | 3.17           | 3.17           | 0.33            | 1.76  | 1.74  |      |    |     |       |       |
| Bonferroni optimal power (1)                 | 3.05           | 3.05           | 0.33            | 2     | 1.38  |      |    |     |       |       |
| Bonferroni greedy algorithm                  | 2.86           | 2.86           | 0.33            | 1.67  | 1.53  |      |    |     |       |       |
| minP                                         | 2.94           | 2.94           | 0.31            | 1.62  | 1.62  |      |    |     |       |       |
| Optimal alpha                                | 4.67           | 2.88           | 0.33            | 1.64  | 1.58  | 5456 | 0  | 22  | 160.5 | 1002  |
| Optimal area                                 | 4.25           | 3.37           | 0.33            | 1.98  | 1.72  | 5456 | 0  | 22  | 156.5 | 998   |
| Optimal power (all, $\rho = 0$ )             | 4.54           | 2.82           | 0.33            | 1.59  | 1.56  | 5456 | 0  | 55  | 927   | 8955  |
| Optimal power (all, $\rho = 0.5$ )           | 4.57           | 2.82           | 0.33            | 1.59  | 1.56  | 5456 | 0  | 13  | 66    | 241   |
| Optimal power (EP 1, $\rho = 0$ )            | 4.43           | 2.98           | 0.33            | 2     | 1.32  | 5454 | 2  | 61  | 2446  | 20000 |
| Consonant optimal alpha                      | 3.45           | 3.45           | 0.33            | 1.92  | 1.87  | 5456 | 0  | 0   | 33    | 206   |
| Consonnat optimal area                       | 3.39           | 3.39           | 0.33            | 1.98  | 1.75  | 5456 | 0  | 0   | 33    | 206   |
| Consonant optimal power (all, $\rho = 0$ )   | 3.42           | 3.42           | 0.33            | 1.88  | 1.86  | 5456 | 0  | 0   | 45    | 1008  |
| Consonant optimal power (all, $\rho = 0.5$ ) | 3.42           | 3.42           | 0.33            | 1.89  | 1.87  | 5456 | 0  | 0   | 8     | 71    |
| Consonant optimal power (EP 1, $\rho = 0$ )  | 3.39           | 3.39           | 0.33            | 2     | 1.72  | 5456 | 0  | 0   | 52.5  | 1122  |
| Greedy algorithm                             | 4.13           | 3.35           | 0.33            | 1.88  | 1.81  |      |    |     |       |       |

Table S14: Power with two binary endpoints,  $n = 15$ ,  $\alpha = 0.05$ ,  $p_{1,Trt} = 0.703$ ,  $p_{2,Trt} = 0.297$ ,  $p_{1,Ctr} = 0.297$ ,  $p_{2,Ctr} = 0.297$ ,  $\rho = 0$ .

| Test                                         | $H_1 \cap H_2$ | $H_1$ or $H_2$ | $H_1$ and $H_2$ | $H_1$ | $H_2$ | C    | NC | q50 | q90   | Max   |
|----------------------------------------------|----------------|----------------|-----------------|-------|-------|------|----|-----|-------|-------|
| Bonferroni                                   | 45.3           | 45.3           | 1               | 44.9  | 1.4   |      |    |     |       |       |
| HKT                                          | 45.8           | 45.8           | 1               | 45.4  | 1.4   |      |    |     |       |       |
| Bonferroni optimal alpha                     | 55.9           | 55.9           | 1.2             | 55.2  | 1.9   |      |    |     |       |       |
| Bonferroni optimal power (all)               | 52.8           | 52.8           | 1.2             | 52    | 1.9   |      |    |     |       |       |
| Bonferroni optimal power (1)                 | 60.8           | 60.8           | 1.2             | 60.4  | 1.7   |      |    |     |       |       |
| Bonferroni greedy algorithm                  | 56.3           | 56.3           | 1.2             | 55.8  | 1.7   |      |    |     |       |       |
| minP                                         | 56.3           | 56.3           | 1.2             | 55.8  | 1.7   |      |    |     |       |       |
| Optimal alpha                                | 48.3           | 42.4           | 1.2             | 41.7  | 1.9   | 5456 | 0  | 22  | 160.5 | 1002  |
| Optimal area                                 | 62.6           | 59.1           | 1.2             | 58.4  | 2     | 5456 | 0  | 22  | 156.5 | 998   |
| Optimal power (all, $\rho = 0$ )             | 53.2           | 46.6           | 1.2             | 45.8  | 2     | 5456 | 0  | 55  | 927   | 8955  |
| Optimal power (all, $\rho = 0.5$ )           | 52.7           | 46.2           | 1.2             | 45.4  | 2     | 5456 | 0  | 13  | 66    | 241   |
| Optimal power (EP 1, $\rho = 0$ )            | 69             | 60.9           | 1.2             | 60.2  | 1.9   | 5454 | 2  | 61  | 2446  | 20000 |
| Consonant optimal alpha                      | 57.8           | 57.8           | 1.2             | 57    | 2     | 5456 | 0  | 0   | 33    | 206   |
| Consonnat optimal area                       | 59.2           | 59.2           | 1.2             | 58.4  | 2     | 5456 | 0  | 0   | 33    | 206   |
| Consonant optimal power (all, $\rho = 0$ )   | 59.9           | 59.9           | 1.2             | 59.1  | 2     | 5456 | 0  | 0   | 45    | 1008  |
| Consonant optimal power (all, $\rho = 0.5$ ) | 59.8           | 59.8           | 1.2             | 59    | 2     | 5456 | 0  | 0   | 8     | 71    |
| Consonant optimal power (EP 1, $\rho = 0$ )  | 61.1           | 61.1           | 1.2             | 60.4  | 2     | 5456 | 0  | 0   | 52.5  | 1122  |
| Greedy algorithm                             | 61.8           | 59             | 1.2             | 58.2  | 2     |      |    |     |       |       |



Table S15: Power with two binary endpoints,  $n = 15$ ,  $\alpha = 0.05$ ,  $p_{1,Trt} = 0.703$ ,  $p_{2,Trt} = 0.703$ ,  $p_{1,Ctr} = 0.297$ ,  $p_{2,Ctr} = 0.297$ ,  $\rho = 0$ .

| Test                                         | $H_1 \cap H_2$ | $H_1$ or $H_2$ | $H_1$ and $H_2$ | $H_1$ | $H_2$ | C    | NC | q50 | q90   | Max   |
|----------------------------------------------|----------------|----------------|-----------------|-------|-------|------|----|-----|-------|-------|
| Bonferroni                                   | 69.5           | 69.5           | 34              | 51.8  | 51.8  |      |    |     |       |       |
| HKT                                          | 69.5           | 69.5           | 34              | 51.8  | 51.8  |      |    |     |       |       |
| Bonferroni optimal alpha                     | 81.8           | 81.8           | 36.4            | 59.7  | 58.6  |      |    |     |       |       |
| Bonferroni optimal power (all)               | 81.7           | 81.7           | 36.4            | 59.6  | 58.5  |      |    |     |       |       |
| Bonferroni optimal power (1)                 | 81.8           | 81.8           | 36.4            | 60.4  | 57.8  |      |    |     |       |       |
| Bonferroni greedy algorithm                  | 81.7           | 81.7           | 36.4            | 59.6  | 58.5  |      |    |     |       |       |
| minP                                         | 79.3           | 79.3           | 35.3            | 57.5  | 57.2  |      |    |     |       |       |
| Optimal alpha                                | 91.2           | 82.3           | 36.4            | 59.6  | 59.2  | 5456 | 0  | 22  | 160.5 | 1002  |
| Optimal area                                 | 89.3           | 83.9           | 36.4            | 60.4  | 60    | 5456 | 0  | 22  | 156.5 | 998   |
| Optimal power (all, $\rho = 0$ )             | 93.5           | 83.3           | 36.4            | 59.9  | 59.8  | 5456 | 0  | 55  | 927   | 8955  |
| Optimal power (all, $\rho = 0.5$ )           | 93.5           | 83.3           | 36.4            | 59.9  | 59.8  | 5456 | 0  | 13  | 66    | 241   |
| Optimal power (EP 1, $\rho = 0$ )            | 89.7           | 81.5           | 36.4            | 60.4  | 57.6  | 5454 | 2  | 61  | 2446  | 20000 |
| Consonant optimal alpha                      | 84.2           | 84.2           | 36.4            | 60.4  | 60.3  | 5456 | 0  | 0   | 33    | 206   |
| Consonnat optimal area                       | 84.1           | 84.1           | 36.4            | 60.4  | 60.2  | 5456 | 0  | 0   | 33    | 206   |
| Consonant optimal power (all, $\rho = 0$ )   | 84.3           | 84.3           | 36.4            | 60.4  | 60.3  | 5456 | 0  | 0   | 45    | 1008  |
| Consonant optimal power (all, $\rho = 0.5$ ) | 84.3           | 84.3           | 36.4            | 60.4  | 60.3  | 5456 | 0  | 0   | 8     | 71    |
| Consonant optimal power (EP 1, $\rho = 0$ )  | 84.2           | 84.2           | 36.4            | 60.4  | 60.2  | 5456 | 0  | 0   | 52.5  | 1122  |
| Greedy algorithm                             | 90.2           | 84.1           | 36.4            | 60.3  | 60.2  |      |    |     |       |       |

Table S16: Power with two binary endpoints,  $n = 15$ ,  $\alpha = 0.05$ ,  $p_{1,Trt} = 0.703$ ,  $p_{2,Trt} = 0.703$ ,  $p_{1,Ctr} = 0.297$ ,  $p_{2,Ctr} = 0.297$ ,  $\rho = 0.5$ .

| Test                                         | $H_1 \cap H_2$ | $H_1$ or $H_2$ | $H_1$ and $H_2$ | $H_1$ | $H_2$ | C    | NC | q50 | q90   | Max   |
|----------------------------------------------|----------------|----------------|-----------------|-------|-------|------|----|-----|-------|-------|
| Bonferroni                                   | 61.2           | 61.2           | 41.7            | 51.4  | 51.4  |      |    |     |       |       |
| HKT                                          | 61.2           | 61.2           | 41.7            | 51.4  | 51.4  |      |    |     |       |       |
| Bonferroni optimal alpha                     | 73.9           | 73.9           | 44.5            | 59.8  | 58.7  |      |    |     |       |       |
| Bonferroni optimal power (all)               | 73.8           | 73.8           | 44.5            | 59.7  | 58.6  |      |    |     |       |       |
| Bonferroni optimal power (1)                 | 73.8           | 73.8           | 44.5            | 60.4  | 58    |      |    |     |       |       |
| Bonferroni greedy algorithm                  | 73.8           | 73.8           | 44.5            | 59.7  | 58.6  |      |    |     |       |       |
| minP                                         | 71.9           | 71.9           | 43.4            | 57.7  | 57.6  |      |    |     |       |       |
| Optimal alpha                                | 81.4           | 74             | 44.5            | 59.4  | 59.1  | 5456 | 0  | 22  | 160.5 | 1002  |
| Optimal area                                 | 79             | 75.8           | 44.5            | 60.4  | 59.9  | 5456 | 0  | 22  | 156.5 | 998   |
| Optimal power (all, $\rho = 0$ )             | 81.8           | 74.8           | 44.5            | 59.7  | 59.6  | 5456 | 0  | 55  | 927   | 8955  |
| Optimal power (all, $\rho = 0.5$ )           | 81.9           | 74.5           | 44.5            | 59.6  | 59.4  | 5456 | 0  | 13  | 66    | 241   |
| Optimal power (EP 1, $\rho = 0$ )            | 80.3           | 74.4           | 44.5            | 60.4  | 58.6  | 5454 | 2  | 61  | 2446  | 20000 |
| Consonant optimal alpha                      | 76             | 76             | 44.5            | 60.3  | 60.2  | 5456 | 0  | 0   | 33    | 206   |
| Consonnat optimal area                       | 75.8           | 75.8           | 44.5            | 60.4  | 60    | 5456 | 0  | 0   | 33    | 206   |
| Consonant optimal power (all, $\rho = 0$ )   | 76             | 76             | 44.5            | 60.3  | 60.2  | 5456 | 0  | 0   | 45    | 1008  |
| Consonant optimal power (all, $\rho = 0.5$ ) | 76             | 76             | 44.5            | 60.3  | 60.2  | 5456 | 0  | 0   | 8     | 71    |
| Consonant optimal power (EP 1, $\rho = 0$ )  | 75.8           | 75.8           | 44.5            | 60.4  | 60    | 5456 | 0  | 0   | 52.5  | 1122  |
| Greedy algorithm                             | 78.9           | 75.8           | 44.5            | 60.3  | 60    |      |    |     |       |       |

Table S17: Power with two binary endpoints,  $n = 20$ ,  $\alpha = 0.025$ ,  $p_{1,Trt} = 0.701$ ,  $p_{2,Trt} = 0.299$ ,  $p_{1,Ctr} = 0.299$ ,  $p_{2,Ctr} = 0.299$ ,  $\rho = 0$ .

| Test                                         | $H_1 \cap H_2$ | $H_1$ or $H_2$ | $H_1$ and $H_2$ | $H_1$ | $H_2$ | C     | NC   | q50 | q90   | Max   |
|----------------------------------------------|----------------|----------------|-----------------|-------|-------|-------|------|-----|-------|-------|
| Bonferroni                                   | 54.8           | 54.8           | 0.7             | 54.6  | 0.9   |       |      |     |       |       |
| HKT                                          | 54.9           | 54.9           | 0.7             | 54.7  | 0.9   |       |      |     |       |       |
| Bonferroni optimal alpha                     | 51.6           | 51.6           | 0.7             | 51.1  | 1.2   |       |      |     |       |       |
| Bonferroni optimal power (all)               | 52.6           | 52.6           | 0.7             | 52.1  | 1.2   |       |      |     |       |       |
| Bonferroni optimal power (1)                 | 60.7           | 60.7           | 0.7             | 60.5  | 1     |       |      |     |       |       |
| Bonferroni greedy algorithm                  | 58.7           | 58.7           | 0.7             | 58.5  | 1     |       |      |     |       |       |
| minP                                         | 58.7           | 58.7           | 0.7             | 58.4  | 1     |       |      |     |       |       |
| Optimal alpha                                | 47.2           | 41.4           | 0.7             | 40.9  | 1.2   | 12341 | 0    | 58  | 740   | 10549 |
| Optimal area                                 | 62.5           | 58.5           | 0.7             | 58    | 1.2   | 12341 | 0    | 57  | 732   | 10522 |
| Optimal power (all, $\rho = 0$ )             | 49.9           | 44             | 0.7             | 43.5  | 1.2   | 11662 | 679  | 208 | 9305  | 20000 |
| Optimal power (all, $\rho = 0.5$ )           | 49.4           | 43.4           | 0.7             | 43    | 1.2   | 12341 | 0    | 32  | 257   | 1287  |
| Optimal power (EP 1, $\rho = 0$ )            | 71.1           | 60.6           | 0.7             | 60.2  | 1.1   | 10521 | 1820 | 341 | 20000 | 20000 |
| Consonant optimal alpha                      | 56.1           | 56.1           | 0.7             | 55.6  | 1.2   | 12341 | 0    | 0   | 79    | 1893  |
| Consonnat optimal area                       | 58.4           | 58.4           | 0.7             | 58    | 1.2   | 12341 | 0    | 0   | 78    | 1889  |
| Consonant optimal power (all, $\rho = 0$ )   | 59.2           | 59.2           | 0.7             | 58.7  | 1.2   | 12341 | 0    | 0   | 278   | 7871  |
| Consonant optimal power (all, $\rho = 0.5$ ) | 59.1           | 59.1           | 0.7             | 58.6  | 1.2   | 12341 | 0    | 0   | 26    | 385   |
| Consonant optimal power (EP 1, $\rho = 0$ )  | 60.9           | 60.9           | 0.7             | 60.5  | 1.2   | 12337 | 4    | 0   | 461   | 20000 |
| Greedy algorithm                             | 62.4           | 59.3           | 0.7             | 58.9  | 1.2   |       |      |     |       |       |

Table S18: Power with two binary endpoints,  $n = 20$ ,  $\alpha = 0.025$ ,  $p_{1,Trt} = 0.701$ ,  $p_{2,Trt} = 0.701$ ,  $p_{1,Ctr} = 0.299$ ,  $p_{2,Ctr} = 0.299$ ,  $\rho = 0$ .

| Test                                         | $H_1 \cap H_2$ | $H_1$ or $H_2$ | $H_1$ and $H_2$ | $H_1$ | $H_2$ | C     | NC   | q50 | q90   | Max   |
|----------------------------------------------|----------------|----------------|-----------------|-------|-------|-------|------|-----|-------|-------|
| Bonferroni                                   | 79.4           | 79.4           | 36.2            | 57.8  | 57.8  |       |      |     |       |       |
| HKT                                          | 79.4           | 79.4           | 36.2            | 57.8  | 57.8  |       |      |     |       |       |
| Bonferroni optimal alpha                     | 82.1           | 82.1           | 36.6            | 59.4  | 59.3  |       |      |     |       |       |
| Bonferroni optimal power (all)               | 82.4           | 82.4           | 36.6            | 59.6  | 59.4  |       |      |     |       |       |
| Bonferroni optimal power (1)                 | 82             | 82             | 36.6            | 60.5  | 58.1  |       |      |     |       |       |
| Bonferroni greedy algorithm                  | 82             | 82             | 36.5            | 59.3  | 59.2  |       |      |     |       |       |
| minP                                         | 81.6           | 81.6           | 36.4            | 59.2  | 58.9  |       |      |     |       |       |
| Optimal alpha                                | 92             | 82.1           | 36.6            | 59.5  | 59.2  | 12341 | 0    | 58  | 740   | 10549 |
| Optimal area                                 | 91.7           | 84.2           | 36.6            | 60.4  | 60.3  | 12341 | 0    | 57  | 732   | 10522 |
| Optimal power (all, $\rho = 0$ )             | 95.2           | 83.7           | 36.6            | 60.2  | 60.1  | 11662 | 679  | 208 | 9305  | 20000 |
| Optimal power (all, $\rho = 0.5$ )           | 95.2           | 83.7           | 36.6            | 60.2  | 60.1  | 12341 | 0    | 32  | 257   | 1287  |
| Optimal power (EP 1, $\rho = 0$ )            | 89.4           | 81             | 36.6            | 60.5  | 57.1  | 10521 | 1820 | 341 | 20000 | 20000 |
| Consonant optimal alpha                      | 84             | 84             | 36.6            | 60.3  | 60.3  | 12341 | 0    | 0   | 79    | 1893  |
| Consonnat optimal area                       | 84.3           | 84.3           | 36.6            | 60.4  | 60.4  | 12341 | 0    | 0   | 78    | 1889  |
| Consonant optimal power (all, $\rho = 0$ )   | 84.4           | 84.4           | 36.6            | 60.5  | 60.5  | 12341 | 0    | 0   | 278   | 7871  |
| Consonant optimal power (all, $\rho = 0.5$ ) | 84.4           | 84.4           | 36.6            | 60.5  | 60.5  | 12341 | 0    | 0   | 26    | 385   |
| Consonant optimal power (EP 1, $\rho = 0$ )  | 84             | 84             | 36.6            | 60.5  | 60.1  | 12337 | 4    | 0   | 461   | 20000 |
| Greedy algorithm                             | 92.5           | 84.3           | 36.6            | 60.4  | 60.4  |       |      |     |       |       |

Table S19: Power with two binary endpoints,  $n = 20$ ,  $\alpha = 0.025$ ,  $p_{1,T\gamma t} = 0.701$ ,  $p_{2,T\gamma t} = 0.701$ ,  $p_{1,Ctr} = 0.299$ ,  $p_{2,Ctr} = 0.299$ ,  $\rho = 0.5$ .

| Test                                         | $H_1 \cap H_2$ | $H_1$ or $H_2$ | $H_1$ and $H_2$ | $H_1$ | $H_2$ | C     | NC   | q50 | q90   | Max   |
|----------------------------------------------|----------------|----------------|-----------------|-------|-------|-------|------|-----|-------|-------|
| Bonferroni                                   | 71.2           | 71.2           | 44.1            | 57.6  | 57.6  |       |      |     |       |       |
| HKT                                          | 71.2           | 71.2           | 44.1            | 57.6  | 57.6  |       |      |     |       |       |
| Bonferroni optimal alpha                     | 74.6           | 74.6           | 44.5            | 59.6  | 59.5  |       |      |     |       |       |
| Bonferroni optimal power (all)               | 74.5           | 74.5           | 44.5            | 59.6  | 59.4  |       |      |     |       |       |
| Bonferroni optimal power (1)                 | 74.2           | 74.2           | 44.5            | 60.5  | 58.3  |       |      |     |       |       |
| Bonferroni greedy algorithm                  | 73.8           | 73.8           | 44.5            | 59.2  | 59    |       |      |     |       |       |
| minP                                         | 74.4           | 74.4           | 44.5            | 59.5  | 59.3  |       |      |     |       |       |
| Optimal alpha                                | 82.1           | 73.4           | 44.5            | 59.1  | 58.9  | 12341 | 0    | 58  | 740   | 10549 |
| Optimal area                                 | 81.4           | 76             | 44.5            | 60.4  | 60.1  | 12341 | 0    | 57  | 732   | 10522 |
| Optimal power (all, $\rho = 0$ )             | 83.8           | 75.2           | 44.5            | 59.9  | 59.8  | 11662 | 679  | 208 | 9305  | 20000 |
| Optimal power (all, $\rho = 0.5$ )           | 83.8           | 75.1           | 44.5            | 59.9  | 59.8  | 12341 | 0    | 32  | 257   | 1287  |
| Optimal power (EP 1, $\rho = 0$ )            | 81.2           | 73.7           | 44.5            | 60.5  | 57.8  | 10521 | 1820 | 341 | 20000 | 20000 |
| Consonant optimal alpha                      | 75.8           | 75.8           | 44.5            | 60.2  | 60.2  | 12341 | 0    | 0   | 79    | 1893  |
| Consonnat optimal area                       | 76.1           | 76.1           | 44.5            | 60.4  | 60.2  | 12341 | 0    | 0   | 78    | 1889  |
| Consonant optimal power (all, $\rho = 0$ )   | 76.3           | 76.3           | 44.5            | 60.4  | 60.4  | 12341 | 0    | 0   | 278   | 7871  |
| Consonant optimal power (all, $\rho = 0.5$ ) | 76.3           | 76.3           | 44.5            | 60.4  | 60.4  | 12341 | 0    | 0   | 26    | 385   |
| Consonant optimal power (EP 1, $\rho = 0$ )  | 75.9           | 75.9           | 44.5            | 60.5  | 59.9  | 12337 | 4    | 0   | 461   | 20000 |
| Greedy algorithm                             | 81.6           | 76.1           | 44.5            | 60.3  | 60.3  |       |      |     |       |       |
