# Supplementary material for: Optimal exact tests for multiple binary endpoints
Source: arXiv:1612.07561 ancillary file (2016-12-22)
Supplement: Supplementary file 2 [file Supplement_2_Simulation_results_for_three_binary_endpoints.pdf]

## Supplemental material 2

### Simulation results for three binary endpoints

The supplemental tables S20 to S25 show the power for the different closed testing procedures when comparing two treatment groups with respect to three binary endpoints. The power was calculated by simulation. For each scenario, 2000 random data samples were drawn from the assumed multivariate Bernoulli distributions using the function `rmvbin` in the library `bindata` in R [1]. The branch and bound algorithm was used with a maximal number of  $5 \cdot 10^5$  iterations. This was sufficient in the case of correlated endpoints. In scenarios with zero correlation and especially when aiming to maximize the exhaustion of the nominal significance level, in some instances no confirmed optimal solution was found for the rejection region of the global intersection hypothesis test. In these cases the best available feasible, though potentially suboptimal, solution was used.

The tables show the probabilities in percent that the closed testing procedure rejects the global intersection hypothesis  $\cap_{i=1}^3 H_i$ , at least one elementary null hypothesis (Any  $H_i$ ), all elementary hypotheses simultaneously (All  $H_i$ ), or particularly  $H_1$ ,  $H_2$ , or  $H_3$ .

In the table headings,  $n$  is the sample size per group,  $\alpha$  the nominal familywise significance level,  $p_{i,Trt}$  and  $p_{i,Ctrl}$  the success probability in endpoint  $i$  in the treatment and control group, respectively, and  $\rho$  the common product moment correlation between the endpoints.

The proportion of simulated instances in which a confirmed optimal solution was found by the branch and bound algorithm for all four intersection hypothesis tests in the closed testing procedure is given in the two columns labelled C(%). To further quantify the number of required iterations for finding the rejection region of the global intersection hypothesis test, the median (q50), the 90 % quantile (q90) and the maximum of the number of iterations are shown in the last three columns. A value of  $5 \cdot 10^5$  indicates that the respective quantity to achieve an optimal solution would be above  $5 \cdot 10^5$ , but is here bounded by the maximal number of iterations.

For tests optimizing the power, the assumed alternative was identical to the true alternative.

Table S20: Power with three binary endpoints,  $n = 10$ ,  $\alpha = 0.025$ ,  $p_{1,Trt} = 0.254$ ,  $p_{2,Trt} = 0.254$ ,  $p_{3,Trt} = 0.254$ ,  $p_{1,Ctr} = 0.254$ ,  $p_{2,Ctr} = 0.254$ ,  $p_{3,Ctr} = 0.254$ ,  $\rho = 0$ . The calculations are based on 2000 random samples, the maximal number of iterations in the branch and bound algorithm was  $5 \cdot 10^5$ .

| Test                        | $\cap_{i=1}^3 H_i$ | Any $H_i$ | All $H_i$ | $H_1$ | $H_2$ | $H_3$ | C(%) | q50     | q90      | Max   |
|-----------------------------|--------------------|-----------|-----------|-------|-------|-------|------|---------|----------|-------|
| Bonferroni                  | 0.4                | 0.4       | 0         | 0.2   | 0     | 0.1   |      |         |          |       |
| HKT                         | 0.7                | 0.7       | 0         | 0.4   | 0.1   | 0.2   |      |         |          |       |
| Bonferroni optimal alpha    | 1.6                | 1.6       | 0         | 0.6   | 0.6   | 0.4   |      |         |          |       |
| Bonferroni optimal power    | 1.6                | 1.6       | 0         | 0.6   | 0.6   | 0.4   |      |         |          |       |
| Bonferroni greedy algorithm | 1.4                | 1.4       | 0         | 0.7   | 0.4   | 0.3   |      |         |          |       |
| minP                        | 1.2                | 1.2       | 0         | 0.6   | 0.4   | 0.3   |      |         |          |       |
| Optimal alpha               | 2.5                | 0.4       | 0         | 0.1   | 0.1   | 0.2   | 73.3 | 14624.5 | 5e+05    | 5e+05 |
| Optimal area                | 2.2                | 1.4       | 0         | 0.7   | 0.4   | 0.3   | 90.3 | 2970    | 479137.3 | 5e+05 |
| Optimal power               | 2.7                | 0.4       | 0         | 0.2   | 0.1   | 0.2   | 73.3 | 14619.5 | 5e+05    | 5e+05 |
| Greedy algorithm            | 2.1                | 1.3       | 0         | 0.6   | 0.4   | 0.3   |      |         |          |       |

Table S21: Power with three binary endpoints,  $n = 10$ ,  $\alpha = 0.025$ ,  $p_{1,Trt} = 0.254$ ,  $p_{2,Trt} = 0.254$ ,  $p_{3,Trt} = 0.254$ ,  $p_{1,Ctr} = 0.254$ ,  $p_{2,Ctr} = 0.254$ ,  $p_{3,Ctr} = 0.254$ ,  $\rho = 0.5$ . The calculations are based on 2000 random samples, the maximal number of iterations in the branch and bound algorithm was  $5 \cdot 10^5$ .

| Test                        | $\cap_{i=1}^3 H_i$ | Any $H_i$ | All $H_i$ | $H_1$ | $H_2$ | $H_3$ | C(%) | q50 | q90   | Max    |
|-----------------------------|--------------------|-----------|-----------|-------|-------|-------|------|-----|-------|--------|
| Bonferroni                  | 0.4                | 0.4       | 0         | 0.3   | 0     | 0.1   |      |     |       |        |
| HKT                         | 0.6                | 0.6       | 0         | 0.4   | 0.1   | 0.2   |      |     |       |        |
| Bonferroni optimal alpha    | 1.7                | 1.7       | 0         | 0.8   | 0.4   | 0.6   |      |     |       |        |
| Bonferroni optimal power    | 1.7                | 1.7       | 0         | 0.8   | 0.4   | 0.6   |      |     |       |        |
| Bonferroni greedy algorithm | 1.5                | 1.5       | 0         | 0.8   | 0.3   | 0.6   |      |     |       |        |
| minP                        | 1.2                | 1.2       | 0         | 0.6   | 0.2   | 0.6   |      |     |       |        |
| Optimal alpha               | 2.6                | 1.1       | 0         | 0.5   | 0.2   | 0.6   | 99.8 | 10  | 683.2 | 5e+05  |
| Optimal area                | 2.6                | 1.5       | 0         | 0.8   | 0.4   | 0.6   | 100  | 10  | 341   | 425584 |
| Optimal power               | 2.5                | 1         | 0         | 0.4   | 0.2   | 0.5   | 99.8 | 9.5 | 683.4 | 5e+05  |
| Greedy algorithm            | 2.5                | 1.6       | 0         | 0.8   | 0.3   | 0.6   |      |     |       |        |

Table S22: Power with three binary endpoints,  $n = 10$ ,  $\alpha = 0.025$ ,  $p_{1,Trt} = 0.746$ ,  $p_{2,Trt} = 0.254$ ,  $p_{3,Trt} = 0.254$ ,  $p_{1,Ctr} = 0.254$ ,  $p_{2,Ctr} = 0.254$ ,  $p_{3,Ctr} = 0.254$ ,  $\rho = 0$ . The calculations are based on 2000 random samples, the maximal number of iterations in the branch and bound algorithm was  $5 \cdot 10^5$ .

| Test                        | $\cap_{i=1}^3 H_i$ | Any $H_i$ | All $H_i$ | $H_1$ | $H_2$ | $H_3$ | C(%) | q50    | q90     | Max   |
|-----------------------------|--------------------|-----------|-----------|-------|-------|-------|------|--------|---------|-------|
| Bonferroni                  | 21.4               | 21.4      | 0         | 21.4  | 0     | 0     |      |        |         |       |
| HKT                         | 37                 | 37        | 0         | 37    | 0.2   | 0.2   |      |        |         |       |
| Bonferroni optimal alpha    | 34.9               | 34.9      | 0         | 34.2  | 0.4   | 0.5   |      |        |         |       |
| Bonferroni optimal power    | 40.6               | 40.6      | 0         | 40.1  | 0.3   | 0.4   |      |        |         |       |
| Bonferroni greedy algorithm | 40.1               | 40.1      | 0         | 39.8  | 0.2   | 0.4   |      |        |         |       |
| minP                        | 39.7               | 39.7      | 0         | 39.4  | 0.2   | 0.4   |      |        |         |       |
| Optimal alpha               | 42.4               | 22.2      | 0         | 21.8  | 0.4   | 0.2   | 42.8 | 5e+05  | 5e+05   | 5e+05 |
| Optimal area                | 46                 | 39.2      | 0         | 38.7  | 0.5   | 0.4   | 71.8 | 53071  | 5e+05   | 5e+05 |
| Optimal power               | 57.5               | 40.3      | 0         | 40    | 0.3   | 0.2   | 98.8 | 1025.5 | 36389.9 | 5e+05 |
| Greedy algorithm            | 44.1               | 38.4      | 0         | 37.8  | 0.4   | 0.5   |      |        |         |       |

Table S23: Power with three binary endpoints,  $n = 10$ ,  $\alpha = 0.025$ ,  $p_{1,Trt} = 0.746$ ,  $p_{2,Trt} = 0.746$ ,  $p_{3,Trt} = 0.746$ ,  $p_{1,Ctr} = 0.254$ ,  $p_{2,Ctr} = 0.254$ ,  $p_{3,Ctr} = 0.254$ ,  $\rho = 0$ . The calculations are based on 2000 random samples, the maximal number of iterations in the branch and bound algorithm was  $5 \cdot 10^5$ .

| Test                        | $\cap_{i=1}^3 H_i$ | Any $H_i$ | All $H_i$ | $H_1$ | $H_2$ | $H_3$ | C(%) | q50    | q90   | Max   |
|-----------------------------|--------------------|-----------|-----------|-------|-------|-------|------|--------|-------|-------|
| Bonferroni                  | 52.4               | 52.4      | 5.7       | 27.7  | 29.8  | 28.5  |      |        |       |       |
| HKT                         | 53.4               | 53.4      | 5.8       | 28.1  | 30.2  | 28.9  |      |        |       |       |
| Bonferroni optimal alpha    | 76                 | 76        | 6.6       | 37.5  | 40    | 39.3  |      |        |       |       |
| Bonferroni optimal power    | 76.1               | 76.1      | 6.6       | 37.5  | 40    | 39.5  |      |        |       |       |
| Bonferroni greedy algorithm | 75.2               | 75.2      | 6.6       | 37.4  | 40.3  | 38.5  |      |        |       |       |
| minP                        | 73.1               | 73.1      | 6.3       | 35.9  | 39    | 37.6  |      |        |       |       |
| Optimal alpha               | 85.8               | 68.5      | 6.6       | 35.5  | 37.5  | 33.8  | 44   | 5e+05  | 5e+05 | 5e+05 |
| Optimal area                | 91.7               | 77.3      | 6.6       | 37.8  | 40.9  | 40    | 81.3 | 31456  | 5e+05 | 5e+05 |
| Optimal power               | 95.8               | 76        | 6.6       | 37    | 40.3  | 39.1  | 64.3 | 132740 | 5e+05 | 5e+05 |
| Greedy algorithm            | 93.3               | 77.4      | 6.6       | 37.8  | 40.9  | 40    |      |        |       |       |

Table S24: Power with three binary endpoints,  $n = 10$ ,  $\alpha = 0.025$ ,  $p_{1,Trt} = 0.746$ ,  $p_{2,Trt} = 0.746$ ,  $p_{3,Trt} = 0.746$ ,  $p_{1,Ctr} = 0.254$ ,  $p_{2,Ctr} = 0.254$ ,  $p_{3,Ctr} = 0.254$ ,  $\rho = 0.5$ . The calculations are based on 2000 random samples, the maximal number of iterations in the branch and bound algorithm was  $5 \cdot 10^5$ .

| Test                        | $\cap_{i=1}^3 H_i$ | Any $H_i$ | All $H_i$ | $H_1$ | $H_2$ | $H_3$ | C(%) | q50  | q90    | Max    |
|-----------------------------|--------------------|-----------|-----------|-------|-------|-------|------|------|--------|--------|
| Bonferroni                  | 43.5               | 43.5      | 17.1      | 30.9  | 30.9  | 31.4  |      |      |        |        |
| HKT                         | 44.1               | 44.1      | 17.1      | 31.1  | 31.2  | 31.6  |      |      |        |        |
| Bonferroni optimal alpha    | 64.6               | 64.6      | 18.1      | 41.2  | 41    | 40.2  |      |      |        |        |
| Bonferroni optimal power    | 64.8               | 64.8      | 18.1      | 41.2  | 40.8  | 40.5  |      |      |        |        |
| Bonferroni greedy algorithm | 63.9               | 63.9      | 18.1      | 41.1  | 40.9  | 39.6  |      |      |        |        |
| minP                        | 63.6               | 63.6      | 18.1      | 40.4  | 40.5  | 40    |      |      |        |        |
| Optimal alpha               | 74.3               | 59.5      | 18.1      | 38.5  | 38.8  | 38.6  | 99.6 | 43.5 | 3166.7 | 5e+05  |
| Optimal area                | 74.5               | 64        | 18.1      | 41.1  | 40.8  | 40    | 100  | 32   | 608.1  | 180941 |
| Optimal power               | 76.9               | 61.2      | 18.1      | 39.3  | 39.5  | 39.5  | 99.8 | 34   | 1646.1 | 5e+05  |
| Greedy algorithm            | 74.3               | 65.3      | 18.1      | 41.2  | 41.1  | 41    |      |      |        |        |

Table S25: Power with three binary endpoints,  $n = 10$ ,  $\alpha = 0.025$ ,  $p_{1,Trt} = 0.8$ ,  $p_{2,Trt} = 0.7$ ,  $p_{3,Trt} = 0.6$ ,  $p_{1,Ctr} = 0.2$ ,  $p_{2,Ctr} = 0.2$ ,  $p_{3,Ctr} = 0.2$ ,  $\rho = 0.5$ . The calculations are based on 2000 random samples, the maximal number of iterations in the branch and bound algorithm was  $5 \cdot 10^5$ .

| Test                        | $\cap_{i=1}^3 H_i$ | Any $H_i$ | All $H_i$ | $H_1$ | $H_2$ | $H_3$ | C(%) | q50 | q90    | Max    |
|-----------------------------|--------------------|-----------|-----------|-------|-------|-------|------|-----|--------|--------|
| Bonferroni                  | 52.8               | 52.8      | 16.1      | 48.7  | 33.5  | 23    |      |     |        |        |
| HKT                         | 55.9               | 55.9      | 16.1      | 51.3  | 34.6  | 23.2  |      |     |        |        |
| Bonferroni optimal alpha    | 72.5               | 72.5      | 16.5      | 63    | 40.8  | 27.4  |      |     |        |        |
| Bonferroni optimal power    | 73.4               | 73.4      | 16.5      | 64    | 41.2  | 27.1  |      |     |        |        |
| Bonferroni greedy algorithm | 72.3               | 72.3      | 16.5      | 63.4  | 40.7  | 27.1  |      |     |        |        |
| minP                        | 72.5               | 72.5      | 16.4      | 63.2  | 40.5  | 27.2  |      |     |        |        |
| Optimal alpha               | 78.6               | 66        | 16.5      | 57.5  | 38.6  | 27    | 99.5 | 44  | 2717.6 | 5e+05  |
| Optimal area                | 80.6               | 73.5      | 16.5      | 64    | 41.2  | 27.3  | 100  | 36  | 595.2  | 133909 |
| Optimal power               | 84.5               | 72.2      | 16.5      | 63.4  | 40.1  | 27    | 100  | 12  | 144    | 24591  |
| Greedy algorithm            | 79.2               | 73.8      | 16.5      | 64.2  | 41.2  | 27.5  |      |     |        |        |

## References

- [1] Leisch F, Weingessel A, and Hornik K. *bindata: Generation of Artificial Binary Data*, 2012. URL <http://CRAN.R-project.org/package=bindata>. R package version 0.9-19, (accessed 15 November 2016).
